# Supplementary material for: Fast sensor placement by enlarging principle submatrix for large-scale linear inverse problems
Source: arXiv:2110.02540 source file (2021-10-07)
Supplement: Supplementary file 1 [file appendix.tex]

\section{Appendix}
\begin{proof}
 Using Proposition 1 to study the eigenvalues' relationship between matrix $-\bPhi_{\bS_t}$ and its submatrix, we will have
    \begin{equation}
    \lambda_{\min}(-\bPhi_{\bS_{t+1}})\le \frac{(1-2v^2_k)\lambda_{\min}(-\bPhi_{\bS_{t}})-\phi_{jj}v^2_k}{1-v^2_k}\nonumber
  \end{equation}
  where $\v$ is the first eigenvector of matrix $-\bPhi_{\bS_t}$ and $v_k$ is the $k$-th element in $\v$.

According to the property that $\lambda_{\min}(-\A)=-\lambda_{\max}(\A)$, we can derive that
\begin{small}
\begin{equation}\label{eq:largest-eigenvalue0}
-\lambda_{\max}(\bPhi_{\bS_{t+1}})\le \frac{-(1-2v^2_k)\lambda_{\max}(\bPhi_{\bS_{t}})-\phi_{jj}v^2_k}{1-v^2_k}
  \end{equation}
  \end{small}
Further, the first eigenvector of $-\bPhi_{\bS_t}$ is the last eigenvector of $\bPhi_{\bS_t}$, \textit{i.e.}, $\v=\p$, so equation \eqref{eq:largest-eigenvalue0} is equal to \eqref{eq:corollary}.
\end{proof}
